# Supplementary material for: Microwave Dressed States and Vacuum Fluctuations in a Superconducting Condensate
Source: arXiv:2511.10364 ancillary file (2025-11-13)
Supplement: Supplementary file 1 [file Supplement.pdf]

# Supplement: Microwave Dressed States and Vacuum Fluctuations in a Superconducting Condensate

Anoop Dhillon[1,*] and A. Hamed Majedi[1,2,3,†]

[1] *Department of Electrical and Computer Engineering, University of Waterloo, Waterloo, Ontario, Canada*

[2] *Department of Physics and Astronomy, University of Waterloo, Waterloo, Ontario, Canada*

[3] *Waterloo Institute of Nanotechnology, Waterloo, Ontario, Canada*

(Dated: November 13, 2025)

This document provides a complete derivation of the theoretical framework outlined in the main text. Although the primary paper presents key results and physical insights, it omits detailed mathematical steps due to spatial constraints. We show these here for completeness.

## LAGRANGIAN DENSITY OF THE SUPERCONDUCTING CONDENSATE

Since the quantized particle excitations of a superconductor are Cooper pairs, which do not have spin, the superconducting condensate can be represented as a charged bosonic gas. The rest mass of its constituent particle excitations is thus $m = 2m_e$, with a charge of $q = 2e$. Consistent with the Ginzburg-Landau theory, the wavefunction of this condensate can be defined by the complex order parameter [1]:

$$\tilde{\psi}\left(\mathbf{x}, t\right) = \sqrt{\rho\left(\mathbf{x}, t\right)} e^{i\theta(\mathbf{x},t)} \tag{1}$$

Where $\rho$ is the particle density, and $\theta$ is the phase of the condensate. Note that the units of this wavefunction are $[\psi] = m^{-3/2}$, which can be used to verify the coefficients of the results derived in the remainder of this report, as we use SI units throughout.

The Lagrangian density of a charged bosonic gas can be represented by that of a complex scalar field, which has the following form [1]:

$$\mathcal{L}_{sc} = \frac{\hbar^2}{mc^2}\left(\partial_o\tilde{\psi}^\dagger\partial_o\tilde{\psi}\right) - \frac{\hbar^2}{m}\left(\nabla\tilde{\psi}^\dagger\cdot\nabla\tilde{\psi}\right) - mc^2\left(\tilde{\psi}^\dagger\tilde{\psi}\right) - V\kappa\left(\tilde{\psi}^\dagger\tilde{\psi}\right)^2 \tag{2}$$

Here, $V$ is the volume of the system, and $\kappa$ is an interaction coefficient that we will define in terms of the electron-phonon scattering of the BCS system in a later part of this derivation.

This effective bosonic field description relies on the physical approximation that the electromagnetic probe wavelength is much longer than the superconducting coherence length, such that the condensate behaves as a collective bosonic entity despite the underlying fermionic constituents [2]. Given the low kinetic energy of particles within the superconducting system, we make a non-relativistic approximation regarding the time-evolution of the wavefunction:

$$\tilde{\psi}\left(\mathbf{x}, t\right) = \psi\left(\mathbf{x}, t\right) e^{-i\frac{mc^2}{\hbar}t} \tag{3}$$

Substituting this into Equation 2, we produce,

$$\mathcal{L}_{sc} = \frac{\hbar^2}{mc^2}\partial_o\psi^\dagger\partial\psi + i\hbar\left(\psi^\dagger\partial_o\psi - \partial_o\psi^\dagger\psi\right) - \frac{\hbar^2}{m}\left(\nabla\psi^\dagger\cdot\nabla\psi\right) - V\kappa\left(\psi^\dagger\psi\right)^2 \tag{4}$$

Due to the inverse particle energy dependence of the first term, we neglect it:

$$\mathcal{L}_{sc} = i\hbar \left(\psi^{\dagger}\partial_o\psi - \partial_o\psi^{\dagger}\psi\right) - \frac{\hbar^2}{m}\left(\nabla\psi^{\dagger}\cdot\nabla\psi\right) - V\kappa\left(\psi^{\dagger}\psi\right)^2 \tag{5}$$

Since the number of bosons within the system must be constant, we define a Lagrange multiplier in terms of the chemical potential ($\mu$) of the system, which can be defined by the electronic Fermi level, for convenience:

$$\therefore \mathcal{L}_{sc} = i\hbar \left(\psi^{\dagger}\partial_o\psi - \partial_o\psi^{\dagger}\psi\right) - \frac{\hbar^2}{m}\left(\nabla\psi^{\dagger}\cdot\nabla\psi\right) - V\kappa\left(\psi^{\dagger}\psi\right)^2 + 2\mu\psi^{\dagger}\psi \tag{6}$$

The factor of 2 in front of the chemical potential is present because the standard chemical potential is defined relative to the number of electrons present, which is twice the number of Cooper pairs. This equation is the Lagrangian density of the superconducting condensate.

## LAGRANGIAN DENSITY OF THE ELECTROMAGNETIC FIELD

As the Lagrangian density of the electromagnetic field is a relatively standard result, we will not belabour its details. In SI units, we give it as [1],

$$\mathcal{L}_{em} = -\frac{1}{4\mu_o}F^{\mu\nu}F_{\mu\nu} = \frac{1}{2}\left(\epsilon_o\mathbf{E}^2 - \frac{1}{\mu_o}\mathbf{B}^2\right) \tag{7}$$

In terms of the electromagnetic four-potential ($A$), we can represent this as,

$$\therefore \mathcal{L}_{em} = \frac{1}{2}\left(\epsilon_o\left(-c\nabla A_o - \partial_o\mathbf{A}\right)^2 - \frac{1}{\mu_o}\left(\nabla\times\mathbf{A}\right)^2\right) \tag{8}$$

Where $cA_o$ is the electric potential, and $\bar{A}$ is the magnetic vector potential.

Note here that we neglect the screening effects of the applied EM field caused by the material system, as we are modelling the condensate in free space. This approach is valid given that superconducting experiments are performed in the microwave region of the spectrum, where the electromagnetic response of these materials is often dominated by the induced motion of their charge carriers, as opposed to their interatomic properties [3].

## LAGRANGIAN DENSITY OF THE INTERACTION

Since the single-particle excitations of the condensate are charged, there must be an interaction between them and the applied EM field. We describe this interaction in terms

of the induced current density as,

$$\mathcal{L}_{int} = -A_{\mu} J^{\mu} \tag{9}$$

We find the magnitude of this current density using Noether's theorem, given the internal $U(1)$ symmetry of the complex scalar field [1], which implies an invariance under the following transformation:

$$\psi \rightarrow \psi' = \psi e^{i\alpha} \tag{10}$$

Therefore, for $\delta\psi = \psi' - \psi$, the Noether current can be derived as,

$$J^{\mu} = \frac{d\mathcal{L}_{sc}}{d\left(\partial_{\mu}\psi\right)} \frac{d\left(\delta\psi\right)}{d\alpha}|_{\alpha=0} + \frac{d\mathcal{L}_{sc}}{d\left(\partial_{\mu}\psi^{\dagger}\right)} \frac{d\left(\delta\psi^{\dagger}\right)}{d\alpha}|_{\alpha=0} \tag{11}$$

Using Equation 6, this can be evaluated as,

$$J^{0} = -cq\left(\psi^{\dagger}\psi - \psi\psi^{\dagger}\right), \quad \mathbf{J} = -\frac{iq\hbar}{m}\left(\nabla\psi\psi^{\dagger} - \nabla\psi^{\dagger}\psi\right) \tag{12}$$

The Lagrangian density describing the interaction is therefore given as,

$$\therefore \mathcal{L}_{int} = cA_{o}q\left(\psi^{\dagger}\psi - \psi\psi^{\dagger}\right) + \mathbf{A}\frac{iq\hbar}{m}\left(\nabla\psi\psi^{\dagger} - \nabla\psi^{\dagger}\psi\right) \tag{13}$$

Assuming the U(1) symmetry to be conserved allows the quantization to be tractable, providing analytical results. However, this symmetry is only conserved when the applied field is weak enough for higher-order contributions to be neglected. This can be seen by considering the gauge-invariant form of this current density:

$$\mathbf{J} = \frac{q}{m}\left((-i\hbar\nabla - qA)\psi\psi^{\dagger} - (-i\hbar\nabla - qA)\psi^{\dagger}\psi\right) \tag{14}$$

From this, a characteristic parameter ($\epsilon$) can be defined as $\epsilon = \frac{qA\xi}{\hbar}$. When $\epsilon \ll 1$, the second-order term can be ignored, as the condensate's amplitude and phase are only weakly perturbed by the applied field.

## QUANTIZATION OF THE LAGRANGIAN

The EM field and the condensate wavefunction will be modelled as independent of each other so that independent eigenbases can be established and modified by their interaction.

To do this, we first convert the Lagrangian density of the system into a Hamiltonian density by deriving the canonical momentum conjugate for each field. For the bosonic condensate, we do this as follows:

$$\Pi^0_{\psi} = \frac{d\mathcal{L}_{sc}}{d\left(\partial_o \psi\right)} = i\hbar\psi^{\dagger}, \quad \Pi^0_{\psi^{\dagger}} = \frac{d\mathcal{L}_{sc}}{d\left(\partial_o \psi^{\dagger}\right)} = -i\hbar\psi \tag{15}$$

Similarly, for the gauge field:

$$\Pi^0_{A_\mu} = \frac{d\mathcal{L}_{em}}{d\left(\partial A_\mu\right)} = \epsilon_o\left(\nabla A_o + \partial_o \mathbf{A}\right) \tag{16}$$

We now derive the Hamiltonian density under the Coulomb gauge:

$$\begin{aligned} \mathcal{H} &= \sum_{\sigma} \Pi^0_{\sigma}\partial_o\sigma - \mathcal{L} \\ \mathcal{H} &= \frac{\hbar^2}{m}\left(\nabla\psi^{\dagger}\cdot\nabla\psi\right) + V\kappa\left(\psi^{\dagger}\psi\right)^2 - \mu\psi^{\dagger}\psi + \frac{\epsilon_o}{2}\left(-\nabla A_o - \partial_o\mathbf{A}\right)^2 \\ &\quad + \frac{1}{2\mu_o}\left(\nabla\times\mathbf{A}\right)^2 - cA_oq\left(\psi^{\dagger}\psi - \psi\psi^{\dagger}\right) - i\mathbf{A}\frac{q\hbar}{m}\left(\nabla\psi\psi^{\dagger} - \nabla\psi^{\dagger}\psi\right) \end{aligned} \tag{17}$$

Given that the superconducting material has no net charge, the scalar potential of the field ($cA_o$) within it is zero:

$$\begin{aligned} \mathcal{H} = \frac{\hbar^2}{m}\left(\nabla\psi^{\dagger}\cdot\nabla\psi\right) + V\kappa\left(\psi^{\dagger}\psi\right)^2 - 2\mu\psi^{\dagger}\psi + \frac{\epsilon_o}{2}\left(\partial_o\mathbf{A}\right)^2 + \frac{1}{2\mu_o}\left(\nabla\times\mathbf{A}\right)^2 \\ - i\mathbf{A}\frac{q\hbar}{m}\left(\nabla\psi\psi^{\dagger} - \nabla\psi^{\dagger}\psi\right) \end{aligned} \tag{18}$$

This result is the Hamiltonian density of the entire system.

We model this Hamiltonian density in the following form:

$$\mathcal{H} = \mathcal{H}_{sc} + \mathcal{H}_{em} + \mathcal{H}_{int} \tag{19}$$

Where,

$$\mathcal{H}_{sc} = \frac{\hbar^2}{m}\left(\nabla\psi^{\dagger}\cdot\nabla\psi\right) + V\kappa\left(\psi^{\dagger}\psi\right)^2 - 2\mu\psi^{\dagger}\psi \tag{20}$$

$$\mathcal{H}_{em} = \frac{\epsilon_o}{2}\left(\partial_o\mathbf{A}\right)^2 + \frac{1}{2\mu_o}\left(\nabla\times\mathbf{A}\right)^2 \tag{21}$$

$$\mathcal{H}_{int} = -i\mathbf{A}\frac{q\hbar}{m}\left(\nabla\psi\psi^{\dagger} - \nabla\psi^{\dagger}\psi\right) \tag{22}$$

as shown in Equations 2, 3, and 4 of our main paper. The Hamiltonian density of the condensate and the EM field can now be quantized independently.

To quantize the EM field, we define the magnetic vector potential in terms of the EM field mode operators:

$$\mathbf{A}\left(\mathbf{x},t\right)=\sum_{k_\lambda}\sqrt{\frac{\hbar}{2V\epsilon_o\omega_\lambda}}\boldsymbol{\epsilon}_{k_\lambda}\left(\hat{a}_{k_\lambda}e^{i(\omega_\lambda t+\mathbf{k}_\lambda\cdot\mathbf{x})}+\hat{a}^\dagger_{k_\lambda}e^{-i(\omega_\lambda t+\mathbf{k}_\lambda\cdot\mathbf{x})}\right) \tag{23}$$

Where $\boldsymbol{\epsilon}_{k_\lambda}$ is the unit polarization vector for the photon with wavevector $k_\lambda$. The subscript of $\lambda$ distinguishes the wavevectors of incident photons from those of particle excitations within the condensate ($k$). Using this definition, we derive the corresponding electric and magnetic field operators:

$$\mathbf{E}\left(\mathbf{x},t\right)=-\partial_o\mathbf{A}\left(\mathbf{x},t\right)=-\sum_{k_\lambda}i\sqrt{\frac{\hbar\omega_\lambda}{2V\epsilon_o}}\boldsymbol{\epsilon}_{k_\lambda}\left(\hat{a}_{k_\lambda}e^{i(\omega_\lambda t+\mathbf{k}_\lambda\cdot\mathbf{x})}-\hat{a}^\dagger_{k_\lambda}e^{-i(\omega_\lambda t+\mathbf{k}_\lambda\cdot\mathbf{x})}\right) \tag{24}$$

$$\mathbf{B}\left(\mathbf{x},t\right)=\nabla\times\mathbf{A}\left(\mathbf{x},t\right)=\sum_{k_\lambda}i\sqrt{\frac{\hbar}{2V\epsilon_o\omega_\lambda}}\left(\mathbf{k}_\lambda\times\boldsymbol{\epsilon}_{k_\lambda}\right)\left(\hat{a}_{k_\lambda}e^{i(\omega_\lambda t+\mathbf{k}_\lambda\cdot\mathbf{x})}+\hat{a}^\dagger_{k_\lambda}e^{-i(\omega_\lambda t+\mathbf{k}_\lambda\cdot\mathbf{x})}\right) \tag{25}$$

The commutation relationship between these EM field operators is given as [4],

$$[\hat{a}_{k_\lambda},\hat{a}^\dagger_{k'_\lambda}]=\delta_{kk'},\quad[\hat{a}_{k_\lambda},\hat{a}_{k'_\lambda}]=0 \tag{26}$$

When acting on number states, they behave as follows [4]:

$$\hat{a}\left|n\right\rangle=\sqrt{n}\left|n-1\right\rangle,\quad\hat{a}\left|0\right\rangle=0,\quad\hat{a}^\dagger\left|n\right\rangle=\sqrt{n+1}\left|n+1\right\rangle \tag{27}$$

We now quantize the condensate by defining it in terms of operators representing single-particle excitations:

$$\psi\left(\mathbf{x},t\right)=\sum_k\sqrt{\frac{mc^2}{V\hbar\omega_k}}\hat{u}_ke^{i\left(\frac{mc^2}{\hbar}t+\mathbf{k}\cdot\mathbf{x}\right)} \tag{28}$$

However, because the velocity of particles in this system is negligible relative to the speed of light $\left(v^2\approx\frac{2k_bT}{m}\approx10^9\ll c^2\right)$, we can approximate the frequency of these particles using their mass energy:

$$E\approx mc^2+\frac{1}{2}mv^2\approx mc^2;\quad\therefore\omega_k\approx\frac{mc^2}{\hbar} \tag{29}$$

Therefore, we can express the quantized representation of the condensate as,

$$\psi\left(\mathbf{x},t\right)=\sum_k\sqrt{\frac{1}{V}}\hat{u}_ke^{i(\omega_kt+\mathbf{k}\cdot\mathbf{x})},\quad\psi^\dagger\left(\mathbf{x},t\right)=\sum_k\sqrt{\frac{1}{V}}\hat{u}^\dagger_ke^{-i(\omega_kt+\mathbf{k}\cdot\mathbf{x})} \tag{30}$$

As stated previously, the single particle excitations of this charged bosonic condensate represent Cooper pairs. In theory, hole-based Cooper pair operators should also be included as the antiparticle excitations of the complex scalar field; however, because they are less often encountered, we neglect their effects. In this representation of the superconducting condensate, the single-particle creation operator ($\hat{u}_k^\dagger$) is related to the BCS creation operators ($\hat{c}_{k\uparrow}^\dagger, \hat{c}_{-k\downarrow}^\dagger$) by,

$$\hat{u}_k^\dagger = \hat{c}_{k\uparrow}^\dagger \hat{c}_{-k\downarrow}^\dagger \tag{31}$$

While the Cooper pairs behave collectively as bosons in the long-wavelength, low-energy limit, this explicit operator form retains the fermionic structure of their constituents ($[\hat{c}_k, \hat{c}_{k'}^\dagger] = \delta_{kk'}$), leading to the modified commutation relation:

$$[\hat{u}_k, \hat{u}_k^\dagger] = \left[\hat{c}_{k\uparrow}\hat{c}_{-k\downarrow}, \hat{c}_{k\uparrow}^\dagger \hat{c}_{-k\downarrow}^\dagger\right] = 1 - \hat{c}_{-k\downarrow}^\dagger \hat{c}_{-k\downarrow} - \hat{c}_{k\uparrow}^\dagger \hat{c}_{k\uparrow} = 1 - \hat{N}_{-k\downarrow} - \hat{N}_{k\uparrow} = 1 - 2\hat{N}_k \tag{32}$$

Where the number operator $\hat{N}_{k\uparrow} = \hat{c}_{k\uparrow}^\dagger \hat{c}_{k\uparrow}$ counts the number of electrons with momentum $k$ and $\uparrow$ spin, meaning that $\hat{N}_k$ counts the number of Cooper pairs with momentum $k$. The implications of this result can be seen when evaluating the action of the creation operator on a state ($|1_k\rangle$) containing a single Cooper pair with certainty:

$$\hat{u}_k \hat{u}_k^\dagger |1_k\rangle = \left(1 - 2\hat{N}_k + \hat{u}_k^\dagger \hat{u}_k\right) |1_k\rangle = (0) |1_k\rangle \tag{33}$$

Therefore, the commutation relation of Equation 32 conveys the fact that the action of the creation operator on a state that already contains a Cooper pair yields a state that is not physically realizable, due to the fermionic nature of its constituents.

Note that in the long-wavelength limit relevant to the photon interactions considered in this work ($q \approx 0$), the distinction between the relative-momentum operator $u_k$ and the centre-of-mass bosonic operator typically associated with bosonic field excitations $b_q$ becomes negligible. In this context, using $u_k$ is preferable, as it allows the underlying fermionic structure of the pair excitation to be preserved, while still capturing the collective, bosonic

response of the condensate. This equivalence can be formally demonstrated as follows:

$$\psi(x,t) = \frac{1}{\sqrt{V}} \sum_q \hat{b}_q e^{i\mathbf{q}\cdot\mathbf{x}} \tag{34}$$

$$\psi(x,t) = \frac{1}{\sqrt{V}} \sum_{q,k} \hat{c}_{k+q/2,\uparrow} \hat{c}_{-k+q/2,\downarrow} e^{i\mathbf{q}\cdot\mathbf{x}} e^{i(\omega_k t + \mathbf{k}\cdot\mathbf{x})} \tag{35}$$

$$[q \approx 0] \tag{36}$$

$$\psi(x,t) = \frac{1}{\sqrt{V}} \sum_{k} \hat{c}_{k,\uparrow} \hat{c}_{-k,\downarrow} e^{i(\omega_k t + \mathbf{k}\cdot\mathbf{x})} \tag{37}$$

$$[\hat{u}_k = \hat{c}_{k,\uparrow} \hat{c}_{-k,\downarrow}] \tag{38}$$

$$\therefore \psi(x,t) = \frac{1}{\sqrt{V}} \sum_{k} \hat{u}_k e^{i(\omega_k t + \mathbf{k}\cdot\mathbf{x})} \tag{39}$$

To analyze the low-energy behaviour of the interacting constituents of the condensate, its interaction Hamiltonian can first be expanded in terms of the wave modes:

$$\mathcal{H}_{Int} = V\kappa \psi^\dagger \psi^\dagger \psi \psi \tag{40}$$

$$\begin{aligned} \mathcal{H}_{Int} = V\kappa & \left( \sum_{k_1} \sqrt{\frac{1}{V}} \hat{u}^\dagger_{k_1} e^{-i(\mathbf{k_1}\cdot\mathbf{x})} \right) \left( \sum_{k_2} \sqrt{\frac{1}{V}} \hat{u}^\dagger_{k_2} e^{-i(\mathbf{k_2}\cdot\mathbf{x})} \right) \cdot \\ & \left( \sum_{q_1} \sqrt{\frac{1}{V}} \hat{u}_{q_1} e^{i(\mathbf{q_1}\cdot\mathbf{x})} \right) \left( \sum_{q_2} \sqrt{\frac{1}{V}} \hat{u}_{q_2} e^{i(\mathbf{q_2}\cdot\mathbf{x})} \right) \end{aligned} \tag{41}$$

$$\mathcal{H}_{Int} = V\kappa \frac{1}{V^2} \left( \sum_{k_1,k_2,q_1,q_2} \hat{u}^\dagger_{k_1} \hat{u}^\dagger_{k_2} \hat{u}_{q_1} \hat{u}_{q_2} e^{-i(\mathbf{k_1}+\mathbf{k_2}-\mathbf{q_1}-\mathbf{q_2})\cdot\mathbf{x}} \right) \tag{42}$$

The spatial integral over volume ($V$) enforces momentum conservation,

$$\int e^{-i(\mathbf{k_1}+\mathbf{k_2}-\mathbf{q_1}-\mathbf{q_2})\cdot\mathbf{x}} dV = V\delta_{\mathbf{k_1}+\mathbf{k_2},\mathbf{q_1}+\mathbf{q_2}} \tag{43}$$

implying $\mathbf{k_1}+\mathbf{k_2} = \mathbf{q_1}+\mathbf{q_2}$. To express this compactly, define $\mathbf{k} = \mathbf{k_1}$, $\mathbf{k}' = \mathbf{k_2}$, and $\mathbf{q}$ such that $\mathbf{q_1} = \mathbf{k} - \mathbf{q}$, $\mathbf{q_2} = \mathbf{k}' + \mathbf{q}$. The interaction Hamiltonian becomes,

$$\mathcal{H}_{Int} = \kappa \sum_{k,k',q} \hat{u}^\dagger_k \hat{u}^\dagger_{k'} \hat{u}_{k+q} \hat{u}_{k-q} \tag{44}$$

Applying the Bogoliubov approximation [5], we separate the macroscopically occupied zero-momentum mode as:

$$\hat{u}_p = \sqrt{n_o}\delta_{p,0} + \delta\hat{u}_p \tag{45}$$

where $n_0$ is the condensate density.

Substituting and retaining terms up to quadratic order in the fluctuations operators ($\delta\hat{u}_{\mathbf{p}}$), we obtain the effective quadratic interaction Hamiltonian:

$$\mathcal{H}_{Int} \approx \kappa n_o \sum_{k,q} \hat{u}_q^\dagger \left(\hat{u}_{k+q} + \hat{u}_{k-q}\right) \tag{46}$$

For clarity, we define an effective interaction coefficient $\kappa' = \kappa n_0$, which absorbs the macroscopic condensate amplitude:

$$\mathcal{H}_{Int} = \kappa' \sum_{k,q} \delta\hat{u}_q^\dagger \left(\delta\hat{u}_{k+q} + \delta\hat{u}_{k-q}\right) \tag{47}$$

This expression describes the scattering of fluctuation modes against the condensate, with momentum transfer $\pm q$.

Using these definitions, we can derive a quantized version of the Hamiltonian from Equation 19, after performing a spatial integration over the volume of the system:

$$\begin{aligned} \therefore H = \sum_{k,k_\lambda,q} & 2\left(\hbar\omega_k - \mu\right)\hat{u}_k^\dagger \hat{u}_k + \kappa' \hat{u}_k^\dagger \hat{u}_{k\pm q} + \frac{\hbar\omega_\lambda}{2}\left(\hat{a}_{k_\lambda}\hat{a}_{k_\lambda}^\dagger + \hat{a}_{k_\lambda}^\dagger \hat{a}_{k_\lambda}\right) \\ & + \sqrt{\frac{q^2c^2\hbar}{V\epsilon_o\omega_\lambda}}\left(\hat{a}_{k_\lambda}e^{i(\omega_\lambda t + \mathbf{k}_\lambda\cdot\mathbf{x})} + \hat{a}_{k_\lambda}^\dagger e^{-i(\omega_\lambda t + \mathbf{k}_\lambda\cdot\mathbf{x})}\right)\left(\hat{u}_k\hat{u}_k^\dagger + \hat{u}_k^\dagger\hat{u}_k\right) \end{aligned} \tag{48}$$

Given our assumption that the wavelength of the incident EM field is much larger than the Pippard coherence length, a dipole approximation ($e^{i\mathbf{k}_\lambda\cdot\mathbf{x}} \approx 1$) can be used to eliminate the spatial dependence from the EM component of the interaction term above:

$$\begin{aligned} \therefore H = \sum_{k,k_\lambda,q} & 2\left(\hbar\omega_k - \mu\right)\hat{u}_k^\dagger \hat{u}_k + \kappa' \hat{u}_k^\dagger \hat{u}_{k\pm q} + \frac{\hbar\omega_\lambda}{2}\left(\hat{a}_{k_\lambda}\hat{a}_{k_\lambda}^\dagger + \hat{a}_{k_\lambda}^\dagger \hat{a}_{k_\lambda}\right) \\ & + \sqrt{\frac{q^2c^2\hbar}{V\epsilon_o\omega_\lambda}}\left(\hat{a}_{k_\lambda}e^{i\omega_\lambda t} + \hat{a}_{k_\lambda}^\dagger e^{-i\omega_\lambda t}\right)\left(\hat{u}_k\hat{u}_k^\dagger + \hat{u}_k^\dagger\hat{u}_k\right) \end{aligned} \tag{49}$$

This is the quantized Hamiltonian of the system, as presented in Equation 7 of the main paper.

In the absence of the EM field, this can be seen to be equivalent to the BCS Hamiltonian using the operator definitions presented in Equation 31 [6]. We use this fact to derive $\kappa'$ in terms of the superconducting gap. Although this derivation will closely follow standard BCS theory, it must be shown, as this allows the results of the field-theoretical formulation

to be related to experimental observations. Firstly, the coherent matter state of the system can be defined in analogy to that of BCS [6]:

$$|\psi_o\rangle = \prod_k \left(u_k + v_k \hat{u}_k^\dagger\right) |0_k\rangle \tag{50}$$

Where $v_k$ and $u_k$ still represent the occupation and non-occupation probabilities for Cooper pairs, respectively, in this mean-field description [6]. We now evaluate the energy of the condensate using the above Hamiltonian in the absence of an EM field:

$$\langle\psi_o|H|\psi_o\rangle = \sum_{k,q} \langle 0_{k\pm q}| \left(u^*_{k\pm q} + v^*_{k\pm q}\hat{u}_{k\pm q}\right) \langle 0_k| \left(u^*_k + v^*_k \hat{u}_k\right) \left[2\left(\hbar\omega_k - \mu\right)\hat{u}_k^\dagger \hat{u}_k + \kappa' \hat{u}_k^\dagger \hat{u}_{k\pm q}\right]$$

$$\cdot \left(u_k |0_k\rangle + v_k |1_k\rangle\right) \left(u_{k\pm q} |0_{k\pm q}\rangle + v_{k\pm q} |1_{k\pm q}\rangle\right)$$

$$\therefore \langle\psi_o|H|\psi_o\rangle = \sum_{k,q} 2\left(\hbar\omega_k - \mu\right) v_k^* v_k + \kappa' v_k^* u^*_{k\pm q} u_k v_{k\pm q} \tag{51}$$

Assuming the occupation probabilities are real, we use the variational method to solve for the relationship between them [6]. Namely, by imposing their normalization through the definition of $u_k = \sin(\theta_k)$ and $v_k = \cos(\theta_k)$, and substituting them into the above result, we recover the following equation:

$$\langle\psi_o|H|\psi_o\rangle = \sum_{k,q} \left(\hbar\omega_k - \mu\right)\left(1 + \cos(2\theta_k)\right) + \frac{\kappa'}{4} \sin(2\theta_k)\sin(2\theta_{k\pm q}) \tag{52}$$

This energy is now minimized with respect to $\theta_k$ to yield,

$$\tan(2\theta_k) = \sum_q \frac{\kappa'}{2} \frac{\sin(2\theta_{k\pm q})}{\left(\hbar\omega_k - \mu\right)} \tag{53}$$

We now make the following energy definitions:

$$\Delta_k = -\frac{1}{2}\sum_q \kappa' \sin(2\theta_{k\pm q}) = -\sum_q \kappa' u_{k\pm q} v_{k\pm q}, \tag{54}$$

$$\xi_k = \hbar\omega_k - \mu, \quad E_k = \sqrt{\Delta_k^2 + \xi_k^2} \tag{55}$$

Such that,

$$\tan(2\theta_k) = -\frac{\Delta_k}{\xi_k}, \quad 2u_k v_k = \sin(2\theta_k) = \frac{\Delta_k}{E_k}, \quad v_k^2 - u_k^2 = \cos(2\theta_k) = -\frac{\xi_k}{E_k} \tag{56}$$

We can now represent the occupation probabilities as,

$$v_k^2 = \frac{1}{2}\left(1 - \frac{\xi_k}{E_k}\right), \quad u_k^2 = \frac{1}{2}\left(1 + \frac{\xi_k}{E_k}\right) \tag{57}$$

The equations above can now be combined to produce a condition for self-consistency, which will provide a physical definition for $\kappa'$:

$$-\Delta_k = \frac{\kappa'}{2} \frac{\Delta_{k\pm q}}{\sqrt{\Delta_{k\pm q}^2 + \xi_k^2}} \tag{58}$$

Consistent with BCS theory, the superconducting gap will be considered to be independent of $k$ for all particles below the critical energy ($\hbar\omega_c$) [6]:

$$-\frac{1}{N(0)\kappa'} = \int_0^{\hbar\omega_c} \frac{d\xi}{\sqrt{\Delta^2 + \xi_k^2}}; \quad \therefore \Delta = \frac{\hbar\omega_c}{\sinh\left(-\frac{1}{N(0)\kappa'}\right)} \tag{59}$$

This expression relates the interaction constant ($\kappa'$) to known values of $\Delta$ for a given material, depending on its density of states at zero temperature ($N(0)$) and critical frequency ($\omega_c$).

## DERIVING THE DRESSED STATES OF THE SYSTEM

Before we identify the dressed states of the system, we need to establish the bare states of the condensate as the eigenstates of the matter Hamiltonian. We do this by considering the energy of the system before and after a single photon is absorbed.

The average energy of the system before photon absorption is equal to that of the coherent matter state combined with the energy of an EM field with $n$ photons. We evaluate this as the expectation value of Equation 49 when acting upon the wavefunction of Equation 50, using the properties of the condensate and EM field operators defined above:

$$\langle \psi_o, n | H | n, \psi_o \rangle = \sum_k \left(2\xi_k v_k^2\right) + \frac{\Delta^2}{\kappa'} + \hbar\omega_\lambda \left(n + \frac{1}{2}\right) \tag{60}$$

Following the absorption of a single photon, the system enters its excited state. Given that we represent the condensate as a charged bosonic gas [1], the Cooper pairs are assumed to remain paired throughout, meaning single-particle excitations are not permitted [7]. Instead, pair-excitations occur [7], in which a Cooper-pair is removed from the collective wavefunction of the condensate but its constituent electrons remain paired by phonon coupling. As defined by BCS [7], these pair excitations can be represented by the replacement of the probabilistically defined Cooper pair as it exists in the condensate (with probability

$|v_k|^2)$, with the definite occupation of its electrons in the $+k$ and $-k$ states and of their holes in the $-k$ and $+k$ states. Representing this excited state using the following notation,

$$|\psi_e\rangle = \prod_{k\neq k_e} \left(u_k + v_k \hat{u_k}^\dagger\right) |0_k\rangle |1_{k_e}\rangle \tag{61}$$

where $|1_{k_e}\rangle = \hat{u}^\dagger_{k_e} |0_{k_e}\rangle$, we calculate the energy of this excited state to be,

$$\begin{aligned}
&\langle \psi_e, n-1|H|n-1, \psi_e\rangle \\
&\quad = \sum_{k\neq k_e} \left(\langle 0_k, 0|H|0, 0_k\rangle\right) + \langle 1_{k_e}, n-1|H|n-1, 1_{k_e}\rangle \\
&\quad = \sum_{k\neq k_e, q} \left(2\xi_k v_k^2 + \kappa' u_k v_{k\pm q} u_{k\pm q} v_k\right) + 2\xi_{k_e} + \hbar\omega_\lambda \left(n - \frac{1}{2}\right) \\
&\quad = \sum_{k,q} \left(2\xi_k v_k^2 + \kappa' u_k v_{k\pm q} u_{k\pm q} v_k\right) - 2\sum_{q} \left(\xi_{k_\lambda} v_{k_\lambda}^2 + \kappa' u_{k_e} v_{k_e\pm q} u_{k_e\pm q} v_{k_e}\right) \\
&\qquad\quad + 4\xi_{k_e} + \hbar\omega_\lambda \left(n - \frac{1}{2}\right) \\
&\quad = \sum_{k} \left(2\xi_k v_k^2\right) + \frac{\Delta^2}{\kappa'} + 4\Delta u_{k_e} v_{k_e} + 2\xi_{k_e}\left(1 - 2v_{k_e}^2\right) + \hbar\omega_\lambda \left(n - \frac{1}{2}\right)
\end{aligned} \tag{62}$$

Here, we note that in stating that the electrons and holes of the Cooper pair are now occupied with certainty, we assume that the thermal occupation probability of those states is unity. As such, this theory considers the system to be at a temperature of 0K.

We now give the nominal energy corresponding to the absorption of a single photon as the difference between the energy of these two bare states:

$$\hbar\omega_{21} \triangleq 4\Delta u_{k_e} v_{k_e} + 2\xi_{k_e}\left(1 - 2v_{k_e}^2\right) = 2\Delta\frac{\Delta}{E_{k_e}} + 2\xi_{k_e}\frac{\xi_{k_e}}{E_{k_e}} = 2\sqrt{\Delta^2 + \xi_{k_e}^2} \tag{63}$$

With $\omega_{21}$ defined as the transition frequency, which is equal to the Cooper-pair excitation frequency given by BCS theory. This is the derivation of the result shown in Equation 9 of the main paper.

The bare states above were defined in accordance with BCS theory, which is why the calculated transition energies were consistent with it. However, if the full Hamiltonian of the system were instead diagonalized explicitly, the resulting eigenstates would incorporate the effects of the interaction term, thus producing dressed states. As will be shown, the energy difference between these dressed states exceeds that of the bare states, but remains consistent with BCS in the appropriate limit.

To find these eigenstates, the total Hamiltonian of Equation 49 can be converted into an atomic Hamiltonian by projecting it into the two-level subspace formed by the bare states defined above. To derive this, we first evaluate the transition dipole moment between the bare states, producing the following result:

$$\langle \psi_e, n | H | \psi_o, n+1 \rangle = \sqrt{\frac{v_{k_e}^2 q^2 c^2 \hbar}{V \epsilon_o \omega_\lambda}} \left( \sqrt{n+1} e^{i \omega_\lambda t} \right) \tag{64}$$

$$\langle \psi_o, n+1 | H | \psi_e, n \rangle = \sqrt{\frac{v_{k_e}^2 q^2 c^2 \hbar}{V \epsilon_o \omega_\lambda}} \left( \sqrt{n+1} e^{-i \omega_\lambda t} \right) \tag{65}$$

Furthermore, by transforming the EM field operators into the interaction picture, and applying the resonant approximation, we express the transition dipole moments as,

$$\langle \psi_e, n | H | \psi_o, n+1 \rangle = \sqrt{\frac{v_{k_e}^2 q^2 c^2 \hbar}{V \epsilon_o \omega_\lambda}} \left( \sqrt{n+1} e^{i \delta t} \right) \tag{66}$$

$$\langle \psi_o, n+1 | H | \psi_e, n \rangle = \sqrt{\frac{v_{k_e}^2 q^2 c^2 \hbar}{V \epsilon_o \omega_\lambda}} \left( \sqrt{n+1} e^{-i \delta t} \right) \tag{67}$$

Where the resonant frequency is defined as, $\delta \stackrel{\triangle}{=} \omega_{21} - \omega_\lambda$. Transforming this back into the Schrodinger picture, we now state the atomic Hamiltonian of the system as shown in Equation 10 of the main paper:

$$H = \hbar \omega_\lambda n + \left( \frac{\hbar \delta}{2} \right) \hat{\sigma}_z + \sqrt{\frac{v_{k_e}^2 q^2 c^2 \hbar}{V \epsilon_o \omega_\lambda}} \left( \sqrt{n+1} \right) \hat{\sigma}_x \tag{68}$$

Where $\hat{\sigma}_z$ and $\hat{\sigma}_x$ are the Pauli Z and X matrices, respectively [4]. We now find the eigenenergies of this system to be,

$$E_o = \hbar \omega_\lambda n - \sqrt{\left( \sqrt{\Delta^2 + \xi_{k_e}^2} - \frac{\hbar \omega_\lambda}{2} \right)^2 + \frac{v_{k_e}^2 q^2 c^2 \hbar}{V \epsilon_o \omega_\lambda} (n+1)} \tag{69}$$

$$E_e = \hbar \omega_\lambda n + \sqrt{\left( \sqrt{\Delta^2 + \xi_{k_e}^2} - \frac{\hbar \omega_\lambda}{2} \right)^2 + \frac{v_{k_e}^2 q^2 c^2 \hbar}{V \epsilon_o \omega_\lambda} (n+1)} \tag{70}$$

which corresponds to the dressed states of this interacting system. We now find the renormalized excitation energy of the system to be,

$$\Delta E = \hbar \sqrt{\left( \frac{2\sqrt{\Delta^2 + \xi_{k_e}^2}}{\hbar} - \omega_\lambda \right)^2 + \frac{4 v_{k_e}^2 q^2 c^2}{V \epsilon_o \hbar \omega_\lambda} (n+1)} \tag{71}$$

In the limit for which the volume of the condensate is large ($V \to \infty$), the resonance energy is minimized at the Fermi level ($\xi_{k_e=k_F} = 0$), where,

$$\Delta E|_{k_e=k_F, V\to\infty} = 2\Delta - \hbar\omega_\lambda \tag{72}$$

which is consistent with the minimum excitation energy of BCS theory [7]. The two equations above are the results shown in Equations 11 and 12 of the main paper.

## SEMI-CLASSICAL DRESSED STATES

In the approach above, we quantized both the condensate and the EM field and derived the dressed states resulting from their interaction. We can also derive a similar effect for the quantized condensate in the presence of a classical EM field.

In this case, the Hamiltonian of Equation 49 is expressed as,

$$H = \sum_{k,k_\lambda,q} 2\left(\hbar\omega_k - \mu\right)\hat{u}_k^\dagger \hat{u}_k + \kappa' \hat{u}_k^\dagger \hat{u}_{k\pm q} + \mathbf{A} qc\sqrt{2}(\hat{u}_k \hat{u}_k^\dagger + \hat{u}_k^\dagger \hat{u}_k) \tag{73}$$

The energies of the bare states remain as we derived them in Equations 60 and 62. However, the transition dipole moment is now given as,

$$\langle \psi_e | H_{int} | \psi_o \rangle = \sqrt{2}\frac{qcv_{k_e}}{\omega_\lambda}|\mathbf{E}| \tag{74}$$

where, $|\mathbf{A}| = \frac{|\mathbf{E}|}{\omega_\lambda}$. As a result, the atomic Hamiltonian of the system is now,

$$H = \hbar\omega n + \left(\frac{\hbar\delta}{2}\right)\hat{\sigma}_z + \sqrt{2}\frac{qcv_{k_e}}{\omega_\lambda}|\mathbf{E}|\hat{\sigma}_x \tag{75}$$

which has the following eigenenergies:

$$E_{1,2} = \hbar\omega_\lambda n \pm \sqrt{\left(\sqrt{\Delta^2 + \xi_{k_e}^2} - \frac{\hbar\omega_\lambda}{2}\right)^2 + \frac{2q^2c^2v_{k_e}^2}{\omega_\lambda^2}|\mathbf{E}|^2} \tag{76}$$

The renormalized excitation energy in this semiclassical regime now becomes,

$$\Delta E_{\text{S-Cl}} = \hbar\sqrt{\left(\frac{2\sqrt{\Delta^2 + \xi_{k_e}^2}}{\hbar} - \omega_\lambda\right)^2 + \frac{8v_{k_e}^2 q^2 c^2}{\hbar^2\omega_\lambda^2}|\mathbf{E}|^2} \tag{77}$$

As stated in equation 18 of the main paper.

## VACUUM FLUCTUATIONS OF THE ELECTRIC FIELD

The effects derived above concern how the presence of the EM field alters the eigenenergies of the condensate. However, the back-action of the condensate on the EM field can also be derived. Since we have applied the minimal coupling approximation, only the electric field of the incident EM wave will be affected by the presence of the condensate. This is because, unlike the magnetic field, we can express the total electric field within the material as the sum of its contributions from the incident wave and that which is produced by the induced charge density: $\mathbf{E}_T = \mathbf{E}_{inc} + \mathbf{E}_J$.

The electric field of the incident EM wave is given directly from Equation 24. We derive the induced electric field from the current density found in Equation 12, using Ampere's law, given that the material is not intrinsically magnetic:

$$
\begin{aligned}
\nabla \times \mathbf{H} &= J + \epsilon_o \partial_o \mathbf{E}_J \\
\mathbf{E}_J &= \sum_{k_\lambda} \frac{i}{\omega_\lambda \epsilon_o} \left( -cq \left( \psi^\dagger \psi - \psi \psi^\dagger \right) - \frac{iq\hbar}{m} \left( \nabla \psi \psi^\dagger - \nabla \psi^\dagger \psi \right) \right) \\
\mathbf{E}_J &= \sum_{k_\lambda, k} - \frac{icq}{V \omega_\lambda \epsilon_o} \left( \hat{u}_k^\dagger \hat{u}_k - \hat{u}_k \hat{u}_k^\dagger \right) + \frac{ikq\hbar}{V \omega_\lambda \epsilon_o m} \left( \hat{u}_k \hat{u}_k^\dagger + \hat{u}_k^\dagger \hat{u}_k \right)
\end{aligned} \tag{78}
$$

We can therefore describe the total electric field as,

$$
\begin{aligned}
\mathbf{E}_T = \sum_{k_\lambda, k} -i \sqrt{\frac{\hbar \omega_\lambda}{2V \epsilon_o}} & \left( \hat{a}_{k_\lambda} e^{i(\omega_\lambda t + \mathbf{k}_\lambda \cdot \mathbf{x})} - \hat{a}_{k_\lambda}^\dagger e^{-i(\omega_\lambda t + \mathbf{k}_\lambda \cdot \mathbf{x})} \right) \\
& - \frac{icq}{V \omega_\lambda \epsilon_o} \left( \hat{u}_k^\dagger \hat{u}_k - \hat{u}_k \hat{u}_k^\dagger \right) + \frac{ikq\hbar}{V \omega_\lambda \epsilon_o m} \left( \hat{u}_k \hat{u}_k^\dagger + \hat{u}_k^\dagger \hat{u}_k \right)
\end{aligned} \tag{79}
$$

We now find the variance of the electric field in the presence of the superconducting ground state by evaluating the expression, $(\Delta \mathbf{E})^2 = \langle \psi_o, n | \mathbf{E}^2 | n, \psi_o \rangle - \langle \psi_o, n | \mathbf{E} | n, \psi_o \rangle^2$.

The first of these terms can be evaluated as,

$$
\begin{aligned}
&\langle\psi_o, n|\mathbf{E}^2|n,\psi_o\rangle \\
&= \langle\psi_o, n|\, \frac{\hbar\omega_\lambda}{2V\epsilon_o}\left(\hat{a}^\dagger\hat{a} + \hat{a}\hat{a}^\dagger\right) \\
&\quad + \left(\frac{icq}{V\omega_\lambda\epsilon_o}\right)^2 \left(\hat{u}^\dagger\hat{u}\hat{u}^\dagger\hat{u} - \hat{u}^\dagger\hat{u}\hat{u}\hat{u}^\dagger - \hat{u}\hat{u}^\dagger\hat{u}^\dagger\hat{u} + \hat{u}\hat{u}^\dagger\hat{u}\hat{u}^\dagger\right) \\
&\quad - 2\frac{ikq\hbar}{V\omega_\lambda m}\frac{icq}{V\omega_\lambda\epsilon_o}\left(-\hat{u}\hat{u}^\dagger\hat{u}\hat{u}^\dagger + \hat{u}^\dagger\hat{u}\hat{u}^\dagger\hat{u}\right) \\
&\quad + \left(\frac{ikq\hbar}{V\omega_\lambda\epsilon_o m}\right)^2 \left(\hat{u}\hat{u}^\dagger\hat{u}\hat{u}^\dagger + \hat{u}^\dagger\hat{u}\hat{u}\hat{u}^\dagger + \hat{u}\hat{u}^\dagger\hat{u}^\dagger\hat{u} + \hat{u}^\dagger\hat{u}\hat{u}^\dagger\hat{u}\right)|n,\psi_o\rangle \\
&= \langle\psi_o, n|\, \frac{\hbar\omega_\lambda}{2V\epsilon_o}(2n+1)|n\rangle\left(u_k|0\rangle + v_k|1\rangle\right) + \left(\frac{icq}{V\omega_\lambda\epsilon_o}\right)^2\left(u_k|0\rangle + v_k|1\rangle\right) \\
&\quad - 2\frac{ikq\hbar}{V\omega_\lambda\epsilon_o m}\frac{icq}{V\omega_\lambda\epsilon_o}\left(-u_k|0\rangle + v_k|1\rangle\right) + \left(\frac{ikq\hbar}{V\omega_\lambda\epsilon_o m}\right)^2\left(u_k|0\rangle + v_k|1\rangle\right) \\
&= \frac{\hbar\omega_\lambda(2n+1)}{2V\epsilon_o} - \left(\frac{cq}{V\omega_\lambda\epsilon_o}\right)^2 + \frac{2ckq^2\hbar}{V^2\omega_\lambda^2\epsilon_o^2 m}\left(v_k^2 - u_k^2\right) - \left(\frac{kq\hbar}{V\omega_\lambda\epsilon_o m}\right)^2
\end{aligned}
\tag{80}
$$

The second term can be evaluated as,

$$
\begin{aligned}
&\langle\psi_o, n|\mathbf{E}|n,\psi_o\rangle^2 \\
&= \langle\psi_o, n|\, \frac{-icq}{V\omega_\lambda\epsilon_o}\left(\hat{u}^\dagger\hat{u} - \hat{u}\hat{u}^\dagger\right) + \frac{ikq\hbar}{V\omega_\lambda\epsilon_o m}\left(\hat{u}\hat{u}^\dagger + \hat{u}^\dagger\hat{u}\right)|n,\psi_o\rangle^2 \\
&= \left(\frac{-icq}{V\omega_\lambda\epsilon_o}\left(v_k^2 - u_k^2\right) + \frac{ikq\hbar}{V\omega_\lambda\epsilon_o m}\right)^2 \\
&= -\left(\frac{cq}{V\omega_\lambda\epsilon_o}\right)^2\left(v_k^2 - u_k^2\right)^2 + \frac{2ckq^2\hbar}{V^2\omega_\lambda^2\epsilon_o^2 m}\left(v_k^2 - u_k^2\right) - \left(\frac{kq\hbar}{V\omega_\lambda\epsilon_o m}\right)^2
\end{aligned}
\tag{81}
$$

As a result, we find the variance of the electric field to be as given by Equation 16 of the main paper:

$$
\begin{aligned}
(\Delta\mathbf{E})^2 &= \frac{\hbar\omega_\lambda}{V\epsilon_o}\left(n + \frac{1}{2}\right) - \left(\frac{cq}{V\omega_\lambda\epsilon_o}\right)^2\left(1 - \left(v_k^2 - u_k^2\right)^2\right) \\
\therefore (\Delta\mathbf{E})^2 &= \frac{\hbar\omega_\lambda}{V\epsilon_o}\left(n + \frac{1}{2}\right) - \left(\frac{cq}{V\omega_\lambda\epsilon_o}\right)^2\left(\frac{\Delta^2}{\Delta^2 + \xi_k^2}\right)
\end{aligned}
\tag{82}
$$

---

* Contact author: a33dhillon@uwaterloo.ca

† Contact author: ahmajedi@uwaterloo.ca

[1] T. Lancaster and S. Blundell, *Quantum Field Theory for the Gifted Amateur*, first edition ed. (Oxford University Press, Oxford, 2014).

[2] J. R. Schrieffer, *Theory of Superconductivity*, rev. print ed., Frontiers in Physics No. 20 (Benjamin/Cummings Pub. Co, Reading, Mass, 1964).

[3] T. Van Duzer, C. W. Turner, and C. W. Turner, *Principles of Superconductive Devices and Circuits* (Elsevier, New York, NY, 1981).

[4] J. C. Garrison and R. Y. Chiao, *Quantum Optics*, Oxford Graduate Texts (Oxford university press, Oxford, 2014).

[5] N. N. Bogolyubov, J. Phys. (USSR) **11**, 23 (1947).

[6] M. Tinkham, *Introduction to Superconductivity*, 2nd ed., Dover Books on Physics (Dover Publ, Mineola, NY, 2015).

[7] J. Bardeen, L. N. Cooper, and J. R. Schrieffer, Phys. Rev. **108**, 1175 (1957).
